# Supplementary material for: Steering of the Skyrmion Hall Angle By Gate Voltage
Source: arXiv:1902.09521 ancillary file (2020-04-21)
Supplement: Supplementary file 1 [file SuppMat.pdf]

# Steering of the Skyrmion Hall Angle By Gate Voltages

## – Supplemental Material –

J. Plettenberg, M. Stier, and M. Thorwart
*I. Institut für Theoretische Physik, Universität Hamburg, Jungiusstraße 9, 20355 Hamburg, Germany*

## I. SPIN TORQUES

Within the *sd*-model, the (bath) Hamiltonian of the itinerant 2D electron gas in the presence of spin-orbit coupling is commonly written as

$$H = \frac{\hbar^2 \boldsymbol{k}^2}{2m} + \boldsymbol{\Omega}\hat{\boldsymbol{\sigma}}\,, \tag{S1}$$

where $m$ is the effective electron mass, $\hat{\boldsymbol{\sigma}}$ the operator of the Pauli matrices and

$$\boldsymbol{\Omega} = J_{\mathrm{sd}}\boldsymbol{n} + \alpha_{\mathrm{R}}(\hat{\boldsymbol{z}} \times \boldsymbol{k}) \tag{S2}$$

a position- and momentum-dependent effective exchange splitting with the exchange coupling $J_{\mathrm{sd}}$ between itinerant electron spins $(\hbar/2)\hat{\boldsymbol{\sigma}}$ and a ferromagnetic background with magnetization direction $\boldsymbol{n}(x, y, t)$ in which the skyrmions (SKs) are formed. $H_{\mathrm{sd}} = J_{\mathrm{sd}}\boldsymbol{n}\hat{\boldsymbol{\sigma}}$ is the well known *sd*-Hamiltonian with the exchange coupling between the magnetic background $\boldsymbol{n}$ and the electron spin $\hat{\boldsymbol{\sigma}}$. The Rashba Hamiltonian $H_{\mathrm{R}} = \alpha_{\mathrm{R}}(\hat{\boldsymbol{z}} \times \boldsymbol{k})\hat{\boldsymbol{\sigma}}$ with the Rashba spin-orbit coupling constant $\alpha_{\mathrm{R}}$ describes the coupling between the electron wave vector $\boldsymbol{k}$ and the electron spin $\hat{\boldsymbol{\sigma}}$ induced by the spin Hall effect and the Edelstein effect [1, 2].

Diagonalization of the bath Hamiltonian yields the dispersion relation

$$E^s_{\boldsymbol{k}} = \frac{\hbar^2 k^2}{2m} + s\sqrt{J^2_{\mathrm{sd}} + \alpha^2_{\mathrm{R}}k^2 + 2J_{\mathrm{sd}}\alpha_{\mathrm{R}}(n_y k_x - n_x k_y)} \tag{S3}$$

of the itinerant electrons with momentum $k = |\boldsymbol{k}|$ for the two energy bands $s = \pm 1$. With the Heisenberg equation of motion we obtain to first order in $d\boldsymbol{\Omega}/dt$ the spin expectation value

$$\langle\hat{\boldsymbol{\sigma}}\rangle_s = s\hat{\boldsymbol{\Omega}} + s\frac{\hbar}{2|\boldsymbol{\Omega}|}\frac{d\hat{\boldsymbol{\Omega}}}{dt} \times \hat{\boldsymbol{\Omega}} \tag{S4}$$

for the two energy bands. To calculate the nonequilibrium spin density in the presence of a current we use the Boltzmann equation

$$\frac{d}{dt}f_s(\boldsymbol{r}, \boldsymbol{k}, t) = -\frac{f_s(\boldsymbol{r}, \boldsymbol{k}, t) - f^{\mathrm{FD}}_s(E^s_{\boldsymbol{k}})}{\tau} \tag{S5}$$

for the probability distribution function $f_s(\boldsymbol{r}, \boldsymbol{k}, t)$ of finding an electron with spin $s$ at the point $\boldsymbol{r}$ with momentum $\boldsymbol{k}$ at time $t$, with the Fermi-Dirac distribution function $f^{\mathrm{FD}}_s(E^s_{\boldsymbol{k}})$. Here, we use a relaxation-time approximation where we assume that the relaxation time $\tau$ is the same for the two energy bands. The Boltzmann equation has the solution

$$f_s(\boldsymbol{r}, \boldsymbol{k}, t) = f^{\mathrm{FD}}_s + \frac{\partial f^{\mathrm{FD}}_s}{\partial \boldsymbol{r}}\dot{\boldsymbol{r}}^s_{\boldsymbol{k}} + \frac{\partial f^{\mathrm{FD}}_s}{\partial \boldsymbol{k}}\dot{\boldsymbol{k}}^s\,, \tag{S6}$$

with $\dot{\boldsymbol{r}}^s_{\boldsymbol{k}} = \partial\epsilon^s_{\boldsymbol{k}}/(\hbar\partial\boldsymbol{k})$ and $\dot{\boldsymbol{k}}^s = -\partial\epsilon^s_{\boldsymbol{k}}/(\hbar\partial\boldsymbol{r}) - eE_x\hat{\boldsymbol{x}}$ where we have applied an electric field in the $x$-direction that is connected to the current density $j_e$ via $E_x = \sigma_e j_e$ with the conductivity $\sigma_e = \pi\hbar^2/(e^2\tau E_{\mathrm{F}})$. $E_{\mathrm{F}}$ denotes the Fermi energy. We then obtain the nonequilibrium spin density

$$\langle\delta\hat{\boldsymbol{\sigma}}\rangle = \int \frac{d\boldsymbol{k}}{(2\pi)^2}\sum_{s=\pm 1}\left(g^1_s + g^2_s\right)\langle\hat{\boldsymbol{\sigma}}\rangle_s\,, \tag{S7}$$

which we solve to second order in $\alpha_{\mathrm{R}}$ and to first order in the spatial derivatives. In order to solve the integral analytically, we assume a large exchange coupling such that $E_{\mathrm{F}} > J_{\mathrm{sd}} > \alpha_{\mathrm{R}}k_{\mathrm{F}}$. This is a very good approximation for physically relevant systems. The adiabatic spin torques then follow as $\boldsymbol{T}^{\mathrm{ad}} = (\gamma J_{\mathrm{sd}}/M_{\mathrm{S}})\boldsymbol{n}\times\langle\delta\hat{\boldsymbol{\sigma}}\rangle$ with the saturation magnetization $M_{\mathrm{S}}$. To zeroth order in $\alpha_{\mathrm{R}}$, the adiabatic spin-transfer torque

$$\boldsymbol{T}^{\mathrm{ad}}_{\mathrm{STT}} = v_{\mathrm{s}}\partial_x\boldsymbol{n} \tag{S8}$$

is recovered. The prefactor $v_{\mathrm{s}} = \gamma P\hbar j_e/(2eM_{\mathrm{S}})$ has the dimension of a velocity and is called effective spin velocity. $P$ denotes the spin polarization. The effective spin velocity is proportional to the external current density $j_e$, so that $v_s$ can easily be tuned. In addition to the spin-transfer torque, we find the adiabatic first- and second-order spin-orbit torques

$$\boldsymbol{T}^{\mathrm{ad}}_1 = \frac{2m\alpha_{\mathrm{R}}}{\hbar^2}v_{\mathrm{s}}(\boldsymbol{n} \times \hat{\boldsymbol{y}}), \tag{S9}$$

$$\begin{aligned}\boldsymbol{T}^{\mathrm{ad}}_2 = \left(\frac{\alpha_{\mathrm{R}}k_{\mathrm{F}}}{J_{\mathrm{sd}}}\right)^2 v_{\mathrm{s}}\Big[&t_x\partial_x\boldsymbol{n} + t_y\partial_y\boldsymbol{n}\\ &+ h_x\boldsymbol{n} \times \hat{\boldsymbol{x}} + h_y\boldsymbol{n} \times \hat{\boldsymbol{y}}\\ &+ d_x\boldsymbol{n} \times (\boldsymbol{n} \times \hat{\boldsymbol{x}}) + d_y\boldsymbol{n} \times (\boldsymbol{n} \times \hat{\boldsymbol{y}})\Big]\end{aligned} \tag{S10}$$

with the coefficients

$$t_x = -\frac{7}{4} + \frac{17}{2}n_y^2 - \frac{11}{4}n_z^2, \tag{S11a}$$

$$t_y = -\frac{17}{2}n_x n_y, \tag{S11b}$$

$$h_x = \frac{1}{2}n_z\partial_x n_y + n_y\partial_x n_z + \frac{1}{2}n_z\partial_y n_x - \frac{1}{2}n_x\partial_y n_z, \tag{S11c}$$

$$h_y = -\frac{3}{2}n_z\partial_x n_x - \frac{1}{2}n_z\partial_y n_y + \frac{1}{2}n_y\partial_y n_z, \tag{S11d}$$

$$d_x = \partial_x n_x + \partial_y n_y, \tag{S11e}$$

$$d_y = \frac{1}{2}\partial_x n_y - \frac{1}{2}\partial_y n_x. \tag{S11f}$$

Damping of the spin dynamics of the localized electrons is described by the Gilbert damping term. Due to effects like impurity scattering or spin-orbit coupling, the itinerant electrons experience damping as well. The corresponding nonadiabatic damping torques are obtained via $\boldsymbol{T}^{\rm nonad} = -\beta(\gamma J_{\rm sd}/M_{\rm S})\boldsymbol{n}\times(\boldsymbol{n}\times\langle\delta\hat{\boldsymbol{\sigma}}\rangle) = -\beta\boldsymbol{n}\times\boldsymbol{T}^{\rm ad}$. Since spin-orbit coupling is one of the main damping sources, the nonadiabatic spin-orbit torques can play a major role for the skyrmion dynamics. This effect is ultimately responsible for the possibility to steer the current-driven SK dynamics.

## II. SECOND-ORDER SPIN-ORBIT TORQUE

In this section, we analyze the effect of spin torques in the second order in the Rashba spin-orbit coupling parameter $\alpha_{\rm R}$. These torques have some very interesting properties, even though their impact is generally rather small.

The spin-transfer torque depends on gradients in the magnetization in the direction of the current only and first-order spin-orbit torques are even independent of any gradients in the magnetization. In contrast to those torques, second-order spin-orbit torques depend on both in-plane magnetization gradients parallel and perpendicular to the current. However, unlike $\boldsymbol{T}_1$, $\boldsymbol{T}_2$ has no contributions independent of magnetization gradients. The terms including gradients perpendicular to the current cannot be captured by common treatments up to first order or by one-dimensional theories. When studying non-centrosymmetric SKs with large magnetization gradients, $\boldsymbol{T}_2$ has to be included as it is the key contribution to the total torques for such gradients.

Second-order spin-orbit torques are inversely proportional to the square of the exchange coupling constant $J_{\rm sd}$, while $\boldsymbol{T}_{\rm STT}$ and $\boldsymbol{T}_1$ are independent of this quantity. Therefore, decreasing $J_{\rm sd}$ increases the magnitude of $\boldsymbol{T}_2$ without affecting the other torques. Most commonly used materials like, e.g., MnSi, that exhibit a stable SK phase, have a large exchange coupling constant that suppresses higher-order spin-orbit torques. Our numerical simulations confirm that it is appropriate to neglect second-order spin-orbit torques in such materials

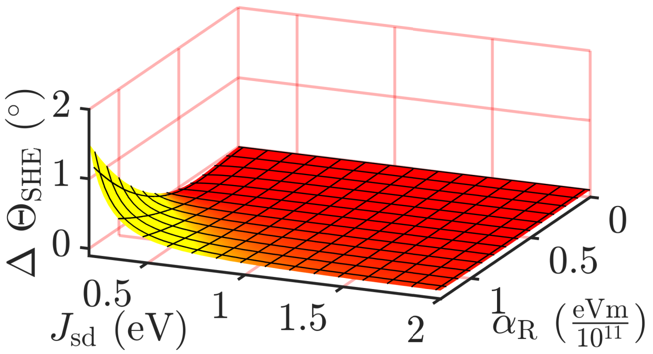


FIG. S1. Difference $\Delta\Theta_{\rm SHE}$ of the SK Hall angle for two sets of calculations, one including and one neglecting second-order spin-orbit torques, as a function of the exchange coupling constant $J_{\rm sd}$ and the Rashba coupling constant $\alpha_{\rm R}$. Material parameters are fixed at $E_{\rm F} = 7$ eV, $\alpha = 0.6$, $\beta = 0.9$. Only for a combination of sufficiently weak exchange coupling and sufficiently large spin-orbit coupling, $\boldsymbol{T}_2$ has a significant impact on the SK Hall angle.

when studying ordinary SKs. This can be seen in the difference plot in Fig. S1, where the impact of $\boldsymbol{T}_2$ on the SK Hall angle $\Theta_{\rm SHE}$ is visualized for a typical set of parameters. The plot shows the difference of two SK Hall angles $\Theta_{\rm SHE}$ resulting of calculations, once including and once neglecting second-order spin-orbit torques. In most commonly used materials, exchange constants of $J_{\rm sd} > 1000$ meV occur. For $J_{\rm sd} > 1000$ meV, it makes practically no difference for $\Theta_{\rm SHE}$ whether second-order torques are included or not. In this case, all relevant torques can also be obtained from one-dimensional theories[3–5] that neglect magnetic gradients perpendicular to the current. One-dimensional models have the advantage that simulations are usually faster and numerically less expensive. Furthermore, it is much easier to extend one-dimensional theories by additional effects such as the backaction of the magnetic background on the spin-polarized current.

## III. CALCULATION OF CURRENT DISTRIBUTION

While the current distribution in simple geometries may be constant this certainly changes in advanced geometries as used in the main part of this Letter. We assume that only the charge current contribution $\mathbf{j}_c$ changes and keep the spin polarization constant. Thus $\mathbf{v}_s \propto \mathbf{j}_c \propto \mathbf{E}$ where $\mathbf{E}$ is the electric field. With the electrical potential $\phi$ get

$$\mathbf{E} = -\nabla\cdot\phi \tag{S12}$$

where $\phi$ itself is calculated by the Laplace equation

$$\triangle\,\phi = 0\ . \tag{S13}$$

We choose von-Neumann boundary conditions such that we have a fixed current flow of $\mathbf{j}_c = j_0\hat{\mathbf{x}}$ on the left and

right (open) edges of the sample and $\mathbf{j}_c = 0$ at the remaining (insulating) edges. The equation itself is solved by numerical standard methods, e.g., by an iterative procedure

$$\phi_{ij} = \frac{1}{4}(\phi_{i-1,j} + \phi_{i+1,j} + \phi_{i,j-1} + \phi_{i,j+1}) \tag{S14}$$

where $\phi$ is replaced by the average of its neighbors on every lattice site $ij$.
Results for the samples used in the main part of the Letter can be seen in Fig. S2. As expected the current distribution changes the most in more complex geometries.


[1] Y. A. Bychkov and E. I. Rashba, J. Phys. C **17**, 6039 (1984).
[2] J. Borge, C. Gorini, G. Vignale, and R. Raimondi, Phys. Rev. B **89** (2014), 10.1103/PhysRevB.89.245443.
[3] M. Stier, R. Egger, and M. Thorwart, Phys. Rev. B **87**, 184415 (2013).
[4] M. Stier, M. Creutzburg, and M. Thorwart, Phys. Rev. B **90**, 014433 (2014).
[5] M. Stier and M. Thorwart, Phys. Rev. B **92**, 220406 (2015).

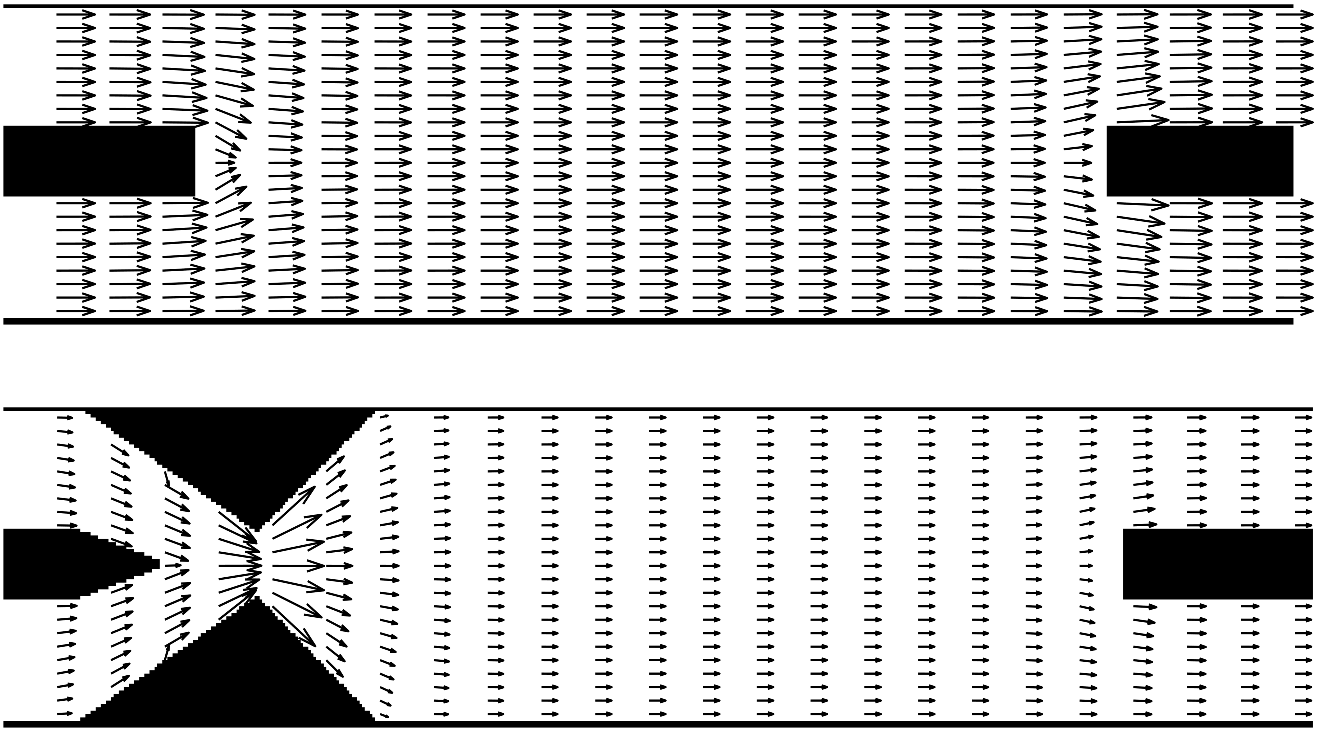

FIG. S2. Current distribution for the sample geometries used in the main part of the Letter. The current flow is fixed to $\mathbf{j}_p = j_0\hat{\mathbf{x}}$ on the left and right hand edges and to $\mathbf{j}_p = 0$ on the remaining edges.
